# Supplementary material for: Improving Implicit Feedback-Based Recommendation through Multi-Behavior Alignment
Source: arXiv:2305.05585 source file (2023-05-09)
Supplement: Supplementary file 1 [file appendix.tex]

%!TEX root = ../main.tex

% \section{APPENDIX}
% The detailed derivation process of the Eq.~\ref{eq:rearrange} as follows:
% \begin{equation} \label{eq:init_kl}
% \begin{aligned}
%     &KL[P(\mathbf{R}_f) \| P(\mathbf{R}_t)] \\
%     &= E_{P(\mathbf{R}_f)}[\log P(\mathbf{R}_f) - \log P(\mathbf{R}_t)] \\
%     &= E_{P(\mathbf{R}_f)}[\log P(\mathbf{R}_f) - \log \frac{P(\mathbf{R}_g)P(\mathbf{R}_t \mid \mathbf{R}_g)}{P(\mathbf{R}_g \mid \mathbf{R}_t)}]\\
%     &= E_{P(\mathbf{R}_f)}[\log P(\mathbf{R}_f) - \log P(\mathbf{R}_g) - \log P(\mathbf{R}_t \mid \mathbf{R}_g) + \log P(\mathbf{R}_g \mid \mathbf{R}_t)]\\
%     &= KL[P(\mathbf{R}_f) \| P(\mathbf{R}_t \mid \mathbf{R}_g)] - \log P(\mathbf{R}_g) + E_{P(\mathbf{R}_f)}[\log P(\mathbf{R}_g \mid \mathbf{R}_t)].
% \end{aligned}    
% \end{equation}
% Then Eq~.\ref{eq:rearrange} can be obtained by rearranging Eq.~\ref{eq:init_kl}.
